# Supplementary material for: Weighted-Lasso for Structured Network Inference from Time Course Data
Source: arXiv:0910.1723 source file (2009-12-09)
Supplement: Supplementary file 1 [file appendices.tex]

\section{Proof of Proposition \ref{prop:var1_mle}}\label{app:proof1}

Thanks to the Markov property of $X_t$, the likelihood writes
\begin{equation}
  \mathcal{L}(\mathbf{X}) = \mathbb{P}(X_0) \prod_{t=1}^n \mathbb{P}(X_t|X_{t-1}).
\end{equation}

Assume for  the sake  of simplicity, yet  with no loss  of generality,
that $\mathbf{b}  = 0$ and $\mathbf{D}=I_p$.  Since  $X_t$ is governed
by                    \eqref{eq:autoregressive}                    and
$\varepsilon_t\sim\mathcal{N}(0,I_p)$, then
\begin{equation*}
  X_t | X_{t-1} = x \sim \mathcal{N}\left(x\mathbf{A}, I_p \right).
\end{equation*}
Hence,  according  to the  parameters  of  interest $\mathbf{A}$,  the
log-likelihood turns to
\begin{equation*}
  \log \mathcal{L}(\mathbf{X};\mathbf{A}) = C-\frac{1}{2}
  \sum_{t=1}^n \left(    X_t-    X_{t-1}\mathbf{A}\right)^\intercal
  \left( X_t- X_{t-1}\mathbf{A} \right), 
\end{equation*}
where  $C$ does  not  depend  on $\mathbf{A}$.   Using  the fact  that
$\mathbf{a}\mathbf{b}^\intercal                                       =
\mathrm{Tr}(\mathbf{a}\mathbf{b}^\intercal)                           =
\mathrm{Tr}(\mathbf{b}^\intercal\mathbf{a})$   for   $\mathbf{a}$  and
$\mathbf{b}$ column vectors and that  the trace operator is linear, it
writes
\begin{equation*}
  \log \mathcal{L}(\mathbf{X};\mathbf{A}) = C'+\frac{1}{2}\left\{
    2 \mathrm{Tr}\left(\sum_{t=1}^n X_t^\intercal X_{t-1} \mathbf{A}\right) -
    \mathrm{Tr}\left(                   \mathbf{A}^\intercal\sum_{t=1}^n
      X_{t-1}^\intercal X_{t-1} \mathbf{A} \right)\right\}.
\end{equation*}
By  means  of notation  \eqref{eq:variances},  we  get the  equivalent
maximization   problem   \eqref{eq:max_log-likelihood}.    Then,   the
maximum-likelihood estimator (MLE) $\widehat{\mathbf{A}}^\mathrm{mle}$
is obtained by direct differentiation, remembering the differentiation
rules for the trace operator:
\begin{equation*}
  \frac{\partial}{\partial   \mathbf{A}}   \mathrm{Tr}   (\mathbf{V}^{\intercal}
  \mathbf{A})    =    \mathbf{V},   \qquad    \frac{\partial}{\partial
    \mathbf{A}} \mathrm{Tr} (\mathbf{A}^\intercal \mathbf{S} \mathbf{A})
  = 2\mathbf{S}\mathbf{A}.
\end{equation*}
since $\mathbf{S}$ is  symmetric.  Null-gradient condition and problem
concavity leads to the final result.

% This reduces to
% \begin{equation*}
%   \log \mathcal{L}(\mathbf{X};\mathbf{A}) = C'+\frac{1}{2}
%   \sum_{t=1}^n \left(  X_t^\intercal X_{t-1}\mathbf{A} + X_t^\intercal
%     X_{t-1}\mathbf{A} -
%     \mathbf{A}^\intercal X_{t-1}^\intercal  X_{t-1}\mathbf{A} \right).
% \end{equation*}

%%% Local Variables:
%%% mode: latex
%%% TeX-master: "J2C.tex"
%%% End:
